# Supplementary material for: A survey on Adversarial Recommender Systems: from Attack/Defense strategies to Generative Adversarial Networks
Source: arXiv:2005.10322 source file (2020-11-10)
Supplement: Supplementary file 1 [file Appendix.tex]

\section{Appendices}
\begin{table}[!t]
\caption{Collaborative-based Recommender Models.}~\felice{ \textbf{@Yashar: }I think that we can remove this table putting the specification directly in the text in order to solve also the R1.3 comment and also gain half-page} \yashar{completely agree, beside this list is not complete nor related to the core part of the survey, if we wanted to make such a list it should have gone to appendix. I would just remove it to gain space.}
\label{tbl:recommender_models}
\centering
{
\scalebox{0.80}{
\begin{tabular}{L{3.5cm}|L{14cm} |}
\toprule
\multicolumn{1}{l}{\textbf{Recommender Abbr.}} &\multicolumn{1}{c}{\textbf{Description}} \\
\bottomrule
\textbf{Classical RS} & \\    \hline \myrowcolour

MF~\cite{DBLP:journals/computer/KorenBV09} & Matrix Factorization (MF) is the state-of-the-art recommendation model for implicit datasets. \\    \hline

BPR-MF~\cite{DBLP:conf/uai/RendleFGS09}  & Bayesian Personalized Ranking (BPR-MF) is a highly competitive MF-model for item recommendation optimized with a pairwise objective function (BPR). \\    \hline \myrowcolour

FM~\cite{DBLP:conf/icdm/Rendle10} & Factorization Machine (FM) is a generalized MF model that encodes (users, items, features)-interactions into a joint dot-product space. \\  \hline

VBPR~\cite{DBLP:conf/aaai/HeM16} & Visual Bayesian Pairwise Ranking (VBPR) model integrates items' visual features --- extracted by a CNN --- in the BPR-MF preference prediction. \\  \hline 

\textbf{Deep-Learning RS} & \\    \hline \myrowcolour

CDL~\cite{DBLP:conf/kdd/WangWY15} & Collaborative Deep Learning (CDL) is a hybrid model combines the extraction of deep items' features with the collaborative user-item feedbacks.  \\  \hline

AutoRec~\cite{DBLP:conf/www/SedhainMSX15}& AutoRec reconstructs partial user profiles (i.e., item recommendation) based on the reconstruction power of auto-encoders .  \\  \hline \myrowcolour

% CDAE~\cite{DBLP:conf/wsdm/WuDZE16}& Collaborative Denoising Auto-Encoder (CDAE) generalizes latent factor models by learning full-users preferences thanks to the reconstruction from a sub-set of preferences.   \\  \hline

CVAE~\cite{DBLP:conf/kdd/LiS17} & Collaborative Variational Auto-Encoder (CVAE) performs recommendations by learning both deep user-item latent representations from content data and implicit user-item relationships from both content and ratings.  \\  \hline 

RRN~\cite{DBLP:conf/wsdm/WuABSJ17} & Recurrent Recommender Networks (RRN) predicts future user preferences by integrating MF with a Long Short-Term Memory (LSTM) model to capture dynamics.\\  \hline \myrowcolour

NCF~\cite{DBLP:conf/www/HeLZNHC17} & Neural Collaborative Filtering (NCF) learns user-item preference function by replacing the inner product of MF with a neural architecture to extract non-linear relations. \\  

\bottomrule
\end{tabular}}}
\end{table}
