# Supplementary material for: A survey on Adversarial Recommender Systems: from Attack/Defense strategies to Generative Adversarial Networks
Source: arXiv:2005.10322 source file (2020-11-10)
Supplement: Supplementary file 2 [file Sec_Appendix.tex]

\section{Appendices}

\input{Tables/Recommender_Models.tex}
